# Supplementary material for: Reinforcement learning for pursuit and evasion of microswimmers at low Reynolds number
Source: arXiv:2106.08609 ancillary file (2022-03-02)
Supplement: Supplementary file 1 [file supplements.pdf]

# Supplementary material: Reinforcement learning for pursuit and evasion of microswimmers at low Reynolds number


Francesco Borra,[1] Luca Biferale,[2] Massimo Cencini,[3] and Antonio Celani[4]

[1]Dipartimento di Fisica, Università "Sapienza" Piazzale A. Moro 5, I-00185 Rome, Italy
[2]Department of Physics and INFN, University of Rome Tor Vergata, Via della Ricerca Scientifica 1, 00133, Rome, Italy
[3]Istituto dei Sistemi Complessi, CNR, via dei Taurini 19, 00185 Rome, Italy and INFN "Tor Vergata"
[4]Quantitative Life Sciences, The Abdus Salam International Centre for Theoretical Physics - ICTP, Trieste, 34151, Italy


## OUTLINE OF SUPPLEMENTARY INFORMATION

In Sec. I we detail the implementation of the Reinforcement Learning algorithm (including the pseudocode). In Sec. II we briefly comment on different choices of the parameters and on the addition of rotational noise, showing that these variations leave qualitatively unchanged the results presented in main text. Finally, Sec. III contains the captions of the supplementary movies.

## I. DETAILS ON THE IMPLEMENTATION OF REINFORCEMENT LEARNING

As explained in main text, the two agents play a zero-sum game with opposite goals: the pursuer needs to find (i.e. to be at distance $\leq R_c$ from) the evader in the shortest possible time, while the latter needs to remain at distance $> R_c$ from the opponent as long as possible. In order to accomplish their goals they can only act on their angular velocity which can take three discrete values: these constitute the set $\mathcal{A}$ of *actions* $a$ each agent can take (here and in the following we drop any reference to the specific agent unless necessary). At each time $t$ (multiple of the decision time $\tau$) the agent has access to some (partial) observation $o_t$ of the *state* of the *environment* via the perceived gradients of the velocity field which are summarized in the features $\boldsymbol{\mathcal{F}}(o_t)$ (observables and features are discussed in Appendix B of main text). Such features are used to parameterize the *policy* $\pi(a|o)$ of each agent that is the probability to take action $a \in \mathcal{A}$ given the observation $o$, parameterized as a softmax function:

$$\pi(a|o) = \frac{\exp\left(\sum_{i=1}^{N_F} \mathcal{F}_i(o)\xi_{ia}\right)}{\sum_{a' \in \mathcal{A}} \exp\left(\sum_{j=1}^{N_F} \mathcal{F}_j(o)\xi_{ja'}\right)} \,. \tag{1}$$

In the above expression $\boldsymbol{\xi} = \{\xi_{ia}\}_{i=1,N_F\ a\in\mathcal{A}}$ are the parameters defining the policy that the agent needs to (learn) optimize to achieve its goal and $N_F$ the number of features used. Once an action is taken the agents receive a reward. To perform such optimization we will use a *reinforcement learning (RL) scheme* to update the parameters $\boldsymbol{\xi}$, which is specified below. For a detailed introduction to RL we refer the reader to the book [6].

### A. Reinforcement Learning Algorithm

We have now to specify the reinforcement-learning update scheme for the policy $\pi(a|o)$ of the learning agent within each episode. We have used a *natural actor-critic* (NAC) scheme [2] (see also Ref. [3] for a general review on actor-critic algorithms). This choice motivated by the fact that our problem setting basically defines a zero-sum game and in Ref. [4] it has been demonstrated that,in stateless zero-sum games, NAC algorithms are able to reproduce the replicator dynamics and thus to find evolutionary stable solutions to the game.

In a nutshell the basic idea of Actor-Critic algorithms is to learn simultaneously both the policy – *actor* step –and the observation value function $V(o)$ – *critic* step –, the latter corresponds to the expected future reward given a certain observation. Figure S 1 schematically describes the working principle, which can be summarized as follows: The agent gets an observation $o_t$ of the environmental state, picks an action $a_t$ according to the current policy $\pi(a_t|o_t)$, gets a reward $r_t$ (for the reward scheme see main text) and observes the environment again $o_{t+\tau}$ then it

***critic* step:** updates with a bootstrap procedure the approximation of the observation value function that, similarly to $\pi$, is parameterized, using the features of table.I in Appendix B of main text, as

$$V(o) = \sum_{i=1}^{N_F} \mathcal{F}_i(o)\kappa_i \,, \tag{2}$$

where $\boldsymbol{\kappa} = \{\kappa_i\}_{i=1,N_F}$ are the parameters to be optimized. Such optimization is realized using *temporal difference* [6], whose basic idea is to produce a new approximation of $V$ evaluating the difference between the actual reward $r_t$ with the expected value according to the approximation of $V$ based on the previous values of the parameters $\boldsymbol{\kappa}$.

***actor* step:** updates the policy parameter with a gradient ascent algorithm (policy gradient theorem in which $V(o)$ is used as a baseline [6]). To improve convergence, we use gradients covariant with respect to the metrics on the parameters defined by the Fisher information $G$ – *natural gradients* [1, 2]. Such natural gradients are approximated by an auxiliary stochastic process as described in Ref. [2].

### B. Pseudocode

We denote with $\eta_A$, $\eta_C$ the learning rates of the actor and critic, respectively. While $\eta_G$ is the learning rates of the estimator, $g_{ia}$ (depending on feature $i$ and action $a$), of the natural gradients. The following pseudocode describes the whole training and policy updating scheme structure. A sample code of the algorithm can be made available upon reasonable request. Policy and value-function update closely follows the natural actor-critic algorithm 3 of [2], adapted to our partial observability and adversarial setting (see e.g. [5]). Upper indices $p/e$ refer to pursuer and evader respectively.

**Parameter initialization**
$\boldsymbol{\xi}^{p/e} \leftarrow \mathbf{0}\,; \quad \boldsymbol{\kappa}^{p/e} \leftarrow \mathbf{0}\,; \quad \boldsymbol{g}^{p/e} \leftarrow \mathbf{0}$
$\eta_C^p = \eta_C^e \leftarrow \eta_C\,; \quad \eta_G^p = \eta_G^e \leftarrow \eta_G$
**Loop on learning cycles**: $(c = 1, \ldots)$
IF $c$ is ODD $\quad \eta_A^p \leftarrow \eta_A \quad \eta_A^e \leftarrow 0$ i.e. pursuer learns
ELSE $\quad \eta_A^p \leftarrow 0 \quad \eta_A^e \leftarrow \eta_A$ i.e. evader learns
**Loop on episodes**: $(e = 1, M)$
Initialize agents' positions and swimming orientations
observations $o_0^{p/e}$
**Loop on time** $t$: $(\{t \le T_{max}$ OR $t | R(t) \le R_c\})$
pick action $a_t^{p/e} \sim \pi^{p/e}(a_t^{p/e}|o_t^{p/e})$
advance dynamics using Eqs. (1)-(2) of main text from $t$ to $t+\tau$
observations $o_{t+\tau}^{p/e}$
Learning updates based on $o_t^{p/e}, o_{t+\tau}^{p/e}, a_t^{p/e}$:
Compute temporal difference:

$$\delta^{p/e} = \begin{cases} -V^{p/e}(o_t^{p/e}) & \text{if the state is terminal} \\ r_t^{p/e} + V^{p/e}(o_t^{p/e}) - V^{p/e}(o_{t+\tau}^{p/e}) & \text{otherwise.} \end{cases}$$

update parameters:

$$\kappa_i^{p/e} \leftarrow \kappa_i^{p/e} + \eta_C^{p/e}\delta^{p/e}\nabla_{\kappa_i} V^{p/e}$$

$$g_{ib}^{p/e} \leftarrow g_{ib}^{p/e} + \eta_G^{p/e}\left[\delta^{p/e} - \sum_{jc}\nabla_{\alpha_{jc}^{p/e}} \ln \pi^{p/e}(a_t^{p/e}|o_t^{p/e}) g_{jc}^{p/e}\right]\nabla_{\alpha_{ib}^{p/e}} \ln \pi^{p/e}(a_t^{p/e}|o_t^{p/e})$$

$$\xi_{ib}^{p/e} \leftarrow \xi_{ib}^{p/e} + \eta_A^{p/e} g_{ib}^{p/e} - (\xi_{ib}^{p/e}/\xi_0)^3 \qquad (\star)$$

$t \leftarrow t + \tau$

In equation $(\star)$ we have added a cubic regularization term to constrain the dynamics of policy parameter since they would otherwise diverge in norm, preventing efficient adversarial updating. The rationale for our choice is that the cubic term does not interfere with the parameter update for $\|\boldsymbol{\xi}\| \ll \xi_0$ but becomes relevant for $\|\boldsymbol{\xi}\| \gg \xi_0 = 20$. The choice of a soft hypercube rather than hard clipping can partially accommodate different intrinsic scales of the features and was empirically more performing. Note that this regularization breaks the covariant structure but was still performing well.

In table I we summarize the parameters used in the definition of episodes and turns, and the learning rates, which as shown in Ref. [2] should be chosen such that $\eta_A \ll \eta_G \ll \eta_C$ to ensure convergence.

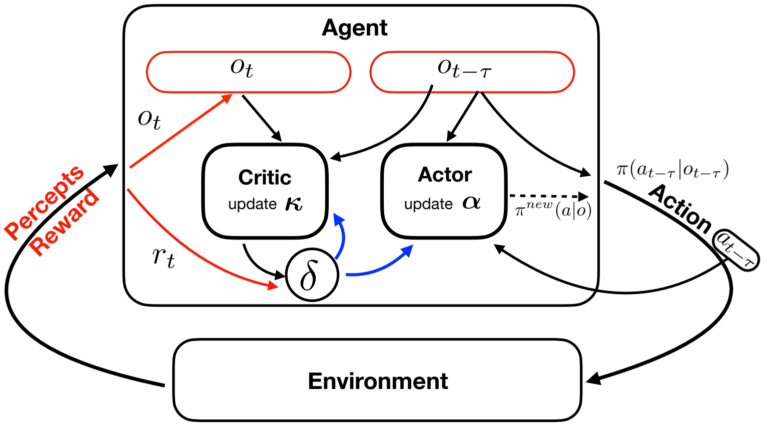


Fig-SI. 1. Pictorial representation of the actor-critic algorithm. The agent interacts with the environment acting on it and modifies its own behavior by looking at the consequences of its actions. Let us start at time $t-\tau$: the agent observes $o_{t-\tau}$ and picks its action $a_{t-\tau}$ according to its current policy $\pi(a_{t-\tau}|o_{t-\tau})$. After decision time $\tau$, the environment responds with a reward $\mathcal{R}_t$ and yields a new observable signal $o_t$. The agent then uses $o_t$, $o_{t-\tau}$ and $\mathcal{R}_t$ to compares the actual outcome of its action with previous expectations (critic) and computes the mismatch $\delta$ (time difference, the circle in the sketch). This mismatch is used to update both expectations about future rewards $V$ and its policy $\pi$. With the new $\pi$, the agent chooses the next action given $o_t$. Color coding: red links show available information, blue links the parameter updating paths.

The dynamics (1)-(2) of main text is integrated with a $4^{th}$ order Runge-Kutta scheme with time-step $dt = 0.02$ time unit, while the decision time is $\tau = 0.1$.

| | | | | | |
|---|---|---|---|---|---|
| $T_{max} = 500$ | $M = 5000$ | $\eta_A = 10^{-5}$ | $\eta_G = 10^{-4}$ | $\eta_C = 10^{-3}$ | $\xi_0 = 20$ |

TABLE I. Parameters used in the reinforcement learning.

## II. TEST WITH DIFFERENT PARAMETERS AND ADDING ROTATIONAL NOISE

In the main text we studied one choice of the parameters (agents' speeds and angular velocities) moreover we did not include any stochastic effect which can affect the dynamics of the microswimmers.

We did studied several variations of the parameters around the values presented in the main text. We always obtained qualitatively similar results: the main pursuit and evasion strategies discussed in Fig.2 of main text were found also in other cases, with some variability in the order in which they are learned which is not surprising given that the learning is intrinsically stochastic. In this section, we show the results for a pursuer faster by a factor 2 than in main text and with larger curvature radius, i.e. $(v_p, \varpi_p) = (0.3, 3)$ and reconsider the example shown in Fig. 2 of main text by adding also stochastic effects in the orientation dynamics. In all cases we keep fixed the force dipole strength to the main text value, i.e. $D_p = D_e = 0.03$.

Figure-SI 2 shows the equivalent of Fig. 2 of main text for the case $(v_p, \varpi_p) = (0.3, 3)$. Also in this case we observe some variability in the history of the rewards and some instabilities in the learning cycles after the second (see Fig-SI. 2a), which again we can interpret in problems related to exploration and/or in the stability of the algorithm as discussed in main text. Panels (b) and (c) display the characteristic mirroring and tailgating strategies learnerd by the pursuer in the first cycle. Differently from the case presented in main text, in its first learning cycle the evader first learn the very effective twirling strategy (panels (h) and (i) show two instances). In the its second turn the pursuer changes its strategy and sometimes is able to win (e.g. panel (d)), its new strategy reveals that in the policy of the evader is also coded other behaviors than twirling such as linear escapes (see panel (j)). For run 1 and 3 anyway, a part from a few intervals for run 3, the evader's policy seems to be very strong or, equivalently, the pursuer has some difficulty in finding an effective counter-strategy. In run2, however, in the second learning cycle of the evader, maybe due to the change of policy of the pursuer, some instability leads to more variegate behaviors and we find capture arches (e) in which the pursuer wins and many episodes in which the evader use the hydrodynamic defense as in (k). These strategies and linear escapes remain for the rest of the cycles, see panels (f,g) and (l,m). Notice that in the same episode the can be combined, e.g. panel (g) shows an instance in which the pursuer can win with an arch

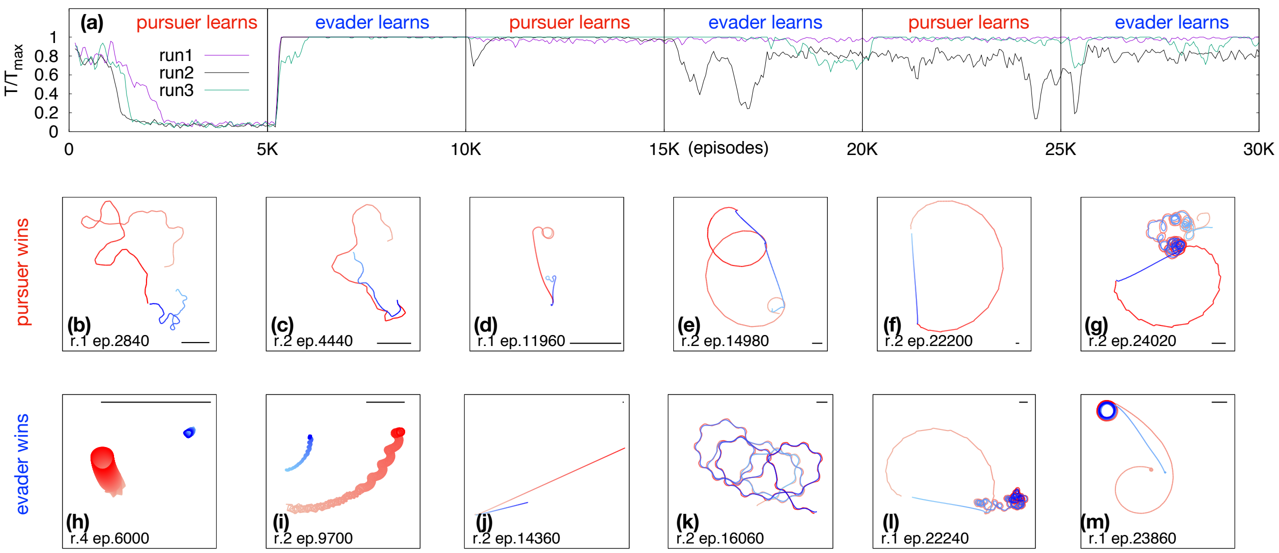


Fig-SI. 2. Co-evolution of pursuit-evasion strategies with $(v_e, \varpi_e) = (0.1, 3)$ and $(v_p, \varpi_p) = (0.3, 3)$, the other parameters as in Fig. 2 of main text. (a) The history of the reward, namely the running average (over 100 episodes) of $T/T_{max}$ for three different realizations as labeled. (b-g) Samples of winning pursuit strategies: (a) mirroring, (b) tailgating, (c) capture upon escape from twirling, (e,f) capture arch similar to panel (d) of Fig.2 main text, (g) successful capture arch after escape from hydrodynamic defense. (h-m) Samples of winning escape strategies: (g,h) two forms of twirling, (j) linear escape, (k) hydrodynamic defense, (l) failed capture arch followed by hydrodynamic defense, (k) similar to (l) but with some variation on the path. Colors coding of the trajectories as in Fig. 2 of main text. Note that the unit length bar is on the bottom/top right for the winning pursuer/evader panels.

after defeating the hydrodynamic defense of the evader, while panels (l) and (m) show two successful hydrodynamic defenses following an attempt of capture of the pursuer.

We also considered a slightly modified dynamics to account for possible rotational noise on the angular dynamics of the microswimmers, i.e. we modified Eq. (2) of main text in

$$\dot{\theta}_\alpha = \Omega_\alpha + \frac{1}{2}\omega^{(\beta)} + \sqrt{2D_r}\eta\,,$$

where $\eta$ is a zero mean, delta-correlated in time Gaussian noise and $D_r$ the rotational diffusion constant. As shown in Fig-SI. 3, obtained with the same parameters of Fig. 1 of main text and $D = 0.025$ we qualitatively found the same results. In particular, notice that the evolution of the reward (Fig-SI. 3a) closely follows the average one of the deterministic case in the first two learning cycles. In particular, panels (b,c) display the typical features of mirroring (b) and tailgating (c), and in panel (d) we show an instance of switching between the two. In the second cycle, where the evader learns, we can recognize the features of the hydrodynamic defense (g) which, due to the rotational noise, however is more curved and irregular with respect to the deterministic case. Panel (h) shows a successful attempt of linear escape which, however, due to the noise is not perfectly linear. Indeed in most of the cases the evader trajectory is irregular and curved so that mirroring is more effecting than in the deterministic case: we can indeed see a failed escape in (e) and a successful one in (i) which is basically indistinguishable from a failed mirroring. Later on (j) the prey learns to use twirling which sometimes fail (f). Possibly due to similar instabilities to those observed in the deterministic case, however, the evader is unable to fix twirling as a winning strategy and in the other cycles we observe a phenomenology similar to that of the second cycle, of these cycles we only show panel (k) which displays an interesting instance in which the pursuer starts with mirroring and the prey is able to make it switch to tailgating which can be contrasted with a hydrodynamic defense.

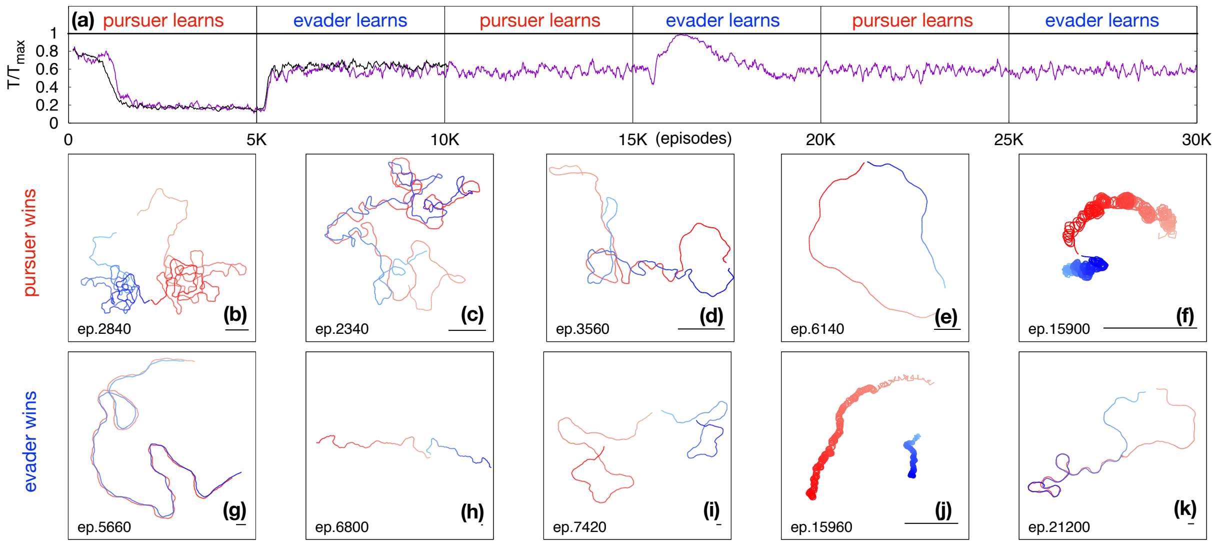


Fig-SI. 3. Co-evolution of pursuit-evasion strategies in the case in which rotational noise with $D_r = 0.025$ is added (values around this one gives similar results within the variability of the learning process which is intrinsically stochastic). (a) The history of the reward, namely the running average (over 100 episodes) of $T/T_{max}$. The purple curve shows one instance of the learning for the case with rotational noise while the black one shows the average, for the first two cycles, of the learning curve of the deterministic case (i.e. the average of run 1, 2 and 3 in Fig.2 of main text. (b-f) Samples of winning pursuit strategies: (a) mirroring, (b) tailgating, (c) switching between the latter two, (e) similar to panel (d) of Fig.2 main text, (f) failed twirling defense. (g-k) Samples of winning escape strategies: (g) hydrodynamic defense, (h) and (i) attempts of linear escapes which due to the noise are almost indistinguishable with mirroring, (j) twirling, (k) successful hydrodynamic defense after a capture attempt with mirroring. Colors coding of the trajectories as in Fig. 2 of main text.

## III. CAPTIONS OF SUPPLEMENTARY MOVIES

**movie1.gif:** Time evolution of pursuer trajectories in run2 episode 6240 (shown in Fig.2h of main text) as seen in the frame of reference of the evader, i.e. with the evader in the origin (the blue circles of size $R_c$ shows the evader position) and oriented with its heading direction along the x-axis. The arrow shows the pursuer relative heading orientation with respect to the evader. Notice that soon the pursuer trajectory becomes basically stationary in this frame of reference, meaning that its speed relative to the prey is basically vanishing.

**movie2.gif:** Similar to movie1.gif but referring to run3 episode 12520 (Fig.2e of main text). Notice that at some instants the trajectory tends to be trapped but suddenly the pursuer finds a way to escape the hydrodynamic trap.

**movie3.gif:** (Top) Evolution of the trajectory of pursuer (red) and evader (blue) in run1 episode 23160 (Fig.2k of main text). (Bottom) evolution of the angle $\Phi_p + \Phi_e$. Notice the approximate switches between mirroring ($\Phi_p + \Phi_e \approx 0$) and tailgating ($\Phi_p + \Phi_e \approx 0$) triggered by the evader turns.


[1] S.-I. Amari. Natural gradient works efficiently in learning. *Neural Comput.*, 10(2):251–276, 1998.

[2] S. Bhatnagar, R. S. Sutton, M. Ghavamzadeh, and M. Lee. Natural actor–critic algorithms. *Automatica*, 45(11):2471–2482, 2009.

[3] I. Grondman, L. Busoniu, G. A. D. Lopes, and R. Babuska. A survey of actor-critic reinforcement learning: Standard and natural policy gradients. *IEEE Trans. Syst. Man. Cybern. Part C*, 42(6):1291–1307, 2012.

[4] D. Hennes, D. Morrill, S. Omidshafiei, R. Munos, J. Perolat, M. Lanctot, A. Gruslys, J.-B. Lespiau, P. Parmas, E. Duenez-Guzman, and K. Tuyls. Neural replicator dynamics. *arXiv:1906.00190 [cs.LG]*, 2019.

[5] T. Jaakkola, S. P. Singh, and M. I. Jordan. Reinforcement learning algorithm for partially observable markov decision problems. In D. S. Touretzky, M. C. Mozer, and M. E. Hasselmo, editors, *Advances in Neural Information Processing Systems*, volume 8, page 345. Morgan Kaufmann Publishers, 1995.

[6] R. S. Sutton and A. G. Barto. *Reinforcement learning: An introduction*. MIT press, 2018.
